# Supplementary material for: Long Phonon Mean Free Paths Observed in Cross-plane Thermal-Conductivity Measurements of Exfoliated Hexagonal Boron Nitride
Source: arXiv:2103.07452 ancillary file (2021-10-08)
Supplement: Supplementary file 1 [file SupportingInformation.pdf]

# Supporting Information

## Long Phonon Mean Free Paths Observed in Cross-plane Thermal-Conductivity Measurements of Exfoliated Hexagonal Boron Nitride

Gabriel R. Jaffe*,[1] Keenan J. Smith,[1] Kenji Watanabe,[2] Takashi Taniguchi,[3] Max G. Lagally,[4] Mark A. Eriksson,[1] and Victor W. Brar[1]

[1]*Department of Physics, University of Wisconsin-Madison, Madison, Wisconsin 53706, USA*

[2]*Research Center for Functional Materials, National Institute for Materials Science, 1-1 Namiki, Tsukuba 305-0044, Japan*

[3]*International Center for Materials Nanoarchitectonics, National Institute for Materials Science, 1-1 Namiki, Tsukuba 305-0044, Japan*

[4]*Department of Materials Science and Engineering, University of Wisconsin-Madison, Madison, Wisconsin 53706, USA*

*Email: gjaffe@wisc.edu

## I. PHONON MEAN FREE PATH EXTRACTION FROM THERMAL CONDUCTIVITY DATA

Here we provide a modification to the procedure for extracting the phonon mean free path spectrum from measurements of thermal conductivity as a function of sample size reported in Ref. 1. The original procedure required that the maximum mean free path point in the Gaussian mesh used in the integral discretization be significantly larger than the thickness of the film for which the thermal conductivity was being calculated. This approach becomes computationally untenable for thick films that would require thousands of points be added to the Gaussian mesh. The modified procedure we report here allows the thermal conductivity of films with large thicknesses to be calculated without adding any additional mesh points. Beginning with Eq. 2 from Ref. 1, we express the effective thermal conductivity $\kappa(L)$ of a thin film of thickness $L$ in terms of the mean free path accumulation function $F(\Lambda) = \int_0^{\Lambda} f(\Lambda')d\Lambda'$ and the Kernel function $K(K_n) = -dS(K_n)/dK_n$ as

$$\kappa(L) = \int_0^{\infty} L^{-1} K(K_n) F(\Lambda) d\Lambda, \tag{1}$$

where $\Lambda$ is the phonon mean free path, $S(K_n)$ is the suppression function, and the Knudsen number is defined as $K_n = \Lambda/L$. We break this integral into two parts

$$\kappa(L) = \int_0^{\Lambda_M} L^{-1} K(K_n) F(\Lambda) d\Lambda + \int_{\Lambda_M}^{\infty} L^{-1} K(K_n) F(\Lambda) d\Lambda. \tag{2}$$

The first integral can be approximated using the Gaussian quadrature. For the second integral, we assume that the maximum phonon mean free path in the Gaussian quadrature mesh, $\Lambda_M$, is chosen to be large enough that the thermal conductivity accumulation function $F(\Lambda_M) \approx 1$. This is a much easier condition to satisfy than $\Lambda_M >> L$ because $L$ can be arbitrarily large. Equation 2 then simplifies to

$$\kappa(L) \approx \sum_{j=1}^{M} w_j L^{-1} K(\frac{\Lambda_j}{L}) F(\Lambda_j) + S(\frac{\Lambda_M}{L}), \tag{3}$$

where $\Lambda_j$ are the quadrature points and $w_j$ are the quadrature weights. This expression is the same as Eq. 3 from Ref. 1 except with the addition of the term $S(\Lambda_M/L)$. We then perform the convex optimization procedure that is outlined in Ref. 1 using the expression given here in Eq. 3 for the thickness-dependent thermal conductivity.

## REFERENCES

[1] A. J. Minnich, "Determining Phonon Mean Free Paths from Observations of Quasiballistic Thermal Transport," Phys. Rev. Lett. **109**, 205901 (2012).
